# Supplementary material for: mRSC: Multi-dimensional Robust Synthetic Control
Source: arXiv:1905.06400 source file (2019-09-23)
Supplement: Supplementary file 1 [file appendix_cricket.tex]

% PROP 2.1 proof
\section{Proofs}
\subsection{Proposition \ref{prop:low-rank}} \label{sec:appendix_proof_prop}
\begin{prop*} %\textbf{(\ref{prop:low-rank})}\\
For any $\varepsilon > 0$, there exists $r = r(\varepsilon, d) \geq 1$ such that matrix $\bfm$ is approximated by a
matrix of rank $r(\varepsilon, d)$ with respect to entry-wise max-norm within $\varepsilon$. That is, there exists
matrix $\bfm^{(r)}$ of rank $r$ such that $\max_{i,j} |m_{ij} - m^{(r)}_{ij}| \leq \varepsilon$. Subsequently, matrix
$\bM^{(r)} = [M^{(r)}_{ij}]$ where $M^{(r)}_{ij} = \sum_{k=1}^j m^{(r)}_{ik}$ is of rank at most $r$ and approximates
$\bM$ such that $\max_{ij} | M_{ij} - M^{(r)}_{ij}| \leq b \varepsilon$. 
\end{prop*}

\begin{proof}
The proof is a straight forward extension of the arguments in \cite{usvt} and \cite{amjadshah1}. 

First, we consider the matrix $\bfm = [m_{ij}], \forall{i} \in [n], \forall{j} \in [b]$. Recall that $m_{ij} = f(\theta_i, \rho_j)$ where $f(\cdot)$ is Lipschitz in its arguments with the Lipschitz constant, $C_f > 0$. We have assumed that the latent parameters belong to a compact space: $[0, 1]^d$, where $d \geq 1$. Given that the number of columns are typically much smaller than the number of rows, i.e. $b << n$, we define a finite covering, $P(\eps)$, such that the following holds: for any $A \in P(\eps)$, whenever $\rho, \rho'$ are two points such that $\rho, \rho' \in A$ we have $| f(\theta_i, \rho) -  f(\theta_i, \rho') | \leq \eps$. Due to the Lipschitzness of the function $f$ and the compactness of any finite subinterval of $[0,1]^d$ it can be shown that $| P(\eps) | \leq C(C_f, d) \eps^{-d}$, where $C(C_f, d)$ is a constant which depends only on the Lipschitz constant, $C_f$, and the dimension of the latent space, $d$.  (see \cite{amjadshah1}).

We now construct the matrix $\bfm^{(r)}$. For latent feature $\rho_j$ corresponding to the column $j \in [b]$, find closest element in $P(\eps)$ and let it be denoted by $p(\rho_j)$. Create the matrix $\bfm^{(r)} = [m_{ij}^{(r)}]$ where $m_{ij}^{(r)}= f(\theta_i, p(\rho_j))$. We note that $\text{rank}(\bfm^{(r)}) = r =  | P(\eps) | \leq C(C_f, d) \eps^{-d} = r(C_f, d, \eps)$. In the manner in which we have constructed $P(\eps)$ and $\bfm^{(r)}$, we know that $m_{ij} - m_{ij}^{(r)} \leq \eps$. Therefore, $\max_{i,j} |m_{ij} - m^{(r)}_{ij}| \leq \varepsilon$, as required.

Next, we consider the cumulative column matrix, $\bM$. First consider that the number of distinct rows (or columns) in $\bfm$ is less than the rank $r = r(C_f, d, \eps)$. Note that each column, $j$, in $\bM$ is generated by taking a sum of all columns $k$, where $1 \leq k \leq j$. Therefore, the relationship between the rows of $\bfm$ is maintained in the rows of $\bM$. This implies that the $\text{rank}(\bM) \leq \text{rank}(\bfm) = r(C_f, d, \eps)$. Finally, given that the last column, $b$, in $\bM$ is the cumulative sum of all columns $k$ where $1 \leq k \leq b$, it must be that $\max_{i,j} |M_{ij} - M^{(r)}_{ij}| \leq b \max_{i,j} |m_{ij} - m^{(r)}_{ij}| = b\varepsilon$.

\end{proof}

% DOMINANCE PROPERTY AND SCALING
\section{Dominance Property} \label{sec:dominance}
We first note that due to the monotonicity properties of runs scored in a cricket innings, we have that if $Y_{ib} > Y_{hb}$ then $Y_{ij} \geq Y_{hj}$ in distribution for two innings $i$ and $h$ and where $j \leq b$. Similarly, if $Y_{ib} < Y_{hb}$ then $Y_{ij} \leq Y_{hj}$ in distribution. We refer to this as the \textit{dominance property} of trajectories. This property tells us that if we have a set of neighbors of the target trajectory where the final score, $Y_{ib}$, is greater (less) than the target score, $t_i$, then the estimated target trajectory for balls $j < b$ will be an upper (lower) bound on the target we are estimating. %This insight allows us to detail in Appendix (Section \ref{sec:dominancescaling}) why choosing trajectories that end {\em at or above} the target and then scaling them all to end exactly at the target is the correct choice for selecting a large enough set of neighbors for each target.
%\section{Dominance Property and Scaling} \label{sec:dominancescaling}
%In Sections \ref{sec:connection_regression} and \ref{sec:dominance} 
In our target revision algorithm, we scale the ``neighbor'' trajectories to all end exactly at the target. If such a scaling is not done, then we expect that a set of neighbors where all innings end above (below) the target will introduce a bias in the estimated trajectory. In Figure \ref{fig:dominancescaling1} we show that this is indeed the case using the data from the second innings of a game played between Pakistan and New Zealand on 01/16/2018. Note that the we use three types of ``neighbors'': innings in the dataset that end up (i) \textbf{above} the target, (ii) \textbf{below} the target and (iii) \textbf{all} innings. We also estimate the targets with and without any scaling. The results confirm our intuition: when no scaling is applied, the neighbors that end up above (below) the target produce an upper-bound (lower-bound) on the estimated target. The all-innings neighbors produces an estimate somewhere in between the upper and lower bounds. However, with scaling all three sets of neighbors produce estimated paths close to each other and far away from the upper/lower bounds. However, note that the (scaled) all innings and (scaled) below innings both produce an estimated path which is higher than the trajectory produced by the above (scaled) neighbors. This appears somewhat counterintuitive. The likely reason for this is that the below neighbor innings (and hence, the all neighbor innings) contain several innings where the chasing team ended up very far from the target either because they got all-out early on in the innings or realized somewhere during the innings that they cannot win and just batted out the rest of the innings without intending to overhaul the target (unfortunately, a common occurrence in past cricket games). When scaling, this introduces a disproportionate positive bias in such innings causing both these sets of neighbors to produce a positively biased estimated target trajectory. The innings that end above the target do not suffer from these problems and for them the scaling makes perfect sense. This experiment conclusively establishes that the choice of neighbors as those innings where the final score is at least as high as the target and then scaling them uniformly is the correct algorithmic choice to produce an estimated target trajectory given the target.

\begin{figure}
	\centering
	\includegraphics[width=0.3\textwidth]{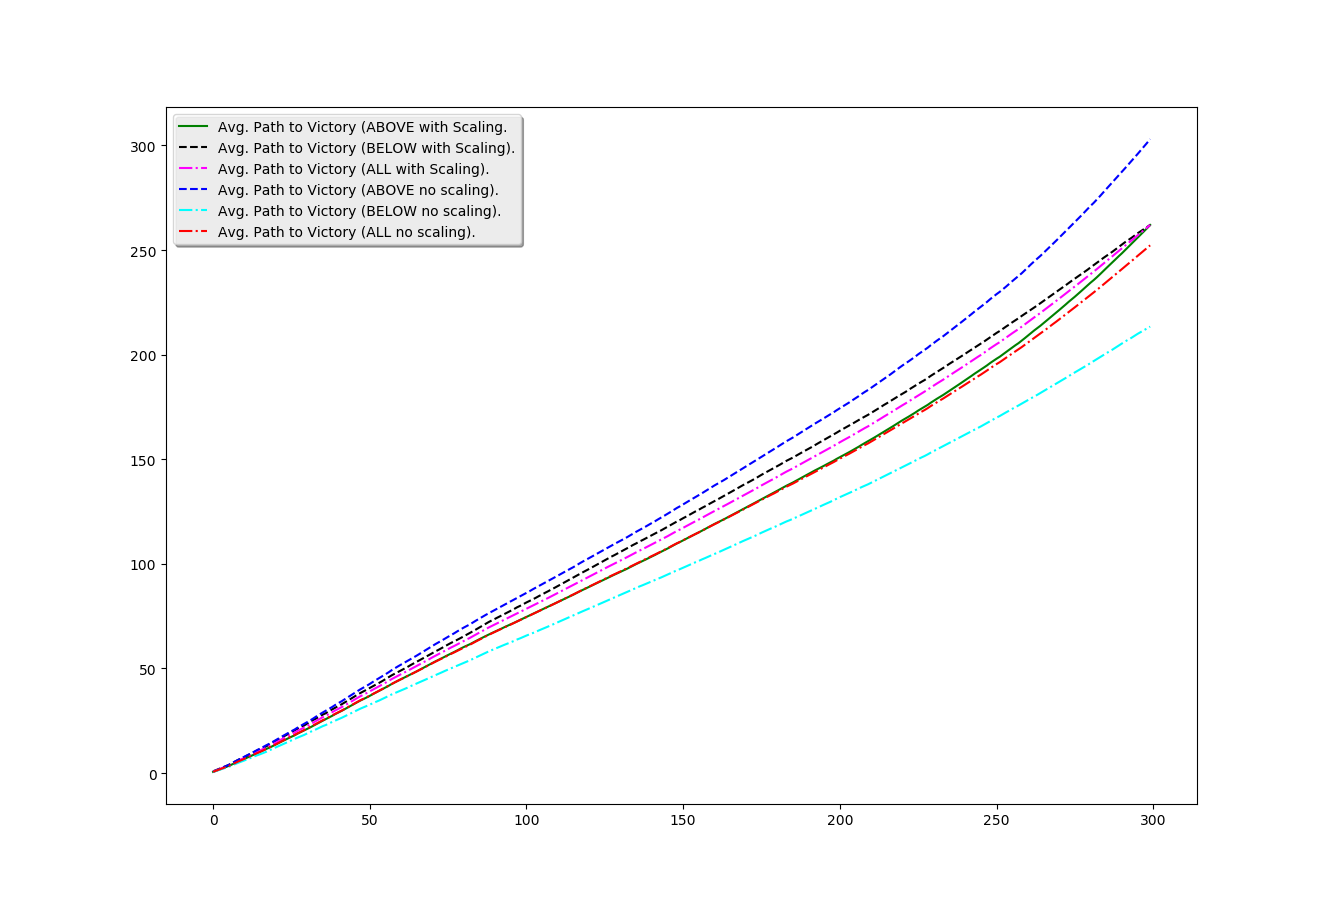}
	\caption{Estimated target trajectories for various sets of ``neighbors'' and scaling.}
	\label{fig:dominancescaling1}
\end{figure}

\section{Forecast Algorithm: Case Studies Continued} \label{sec:appendix_forecastcasestudies}
In the game under considered in Section \ref{sec:forecastcasestudies} (India and Australia at the ICC World Cup 2011), India was able to chase the target down and win the game with relative ease. Figure \ref{fig:aus-ind-2} shows the forecasts at the intervention points of 35, 40 and 45 overs for India's innings. The forecast trajectories are exceptionally close to reality and showcase the predictive ability of the algorithm. Once again notice the rise in score rate towards the late stages of the innings, similar to the first innings. We note that the flatlining of the actual score in the innings (red line) is simply due to the fact that India had won the game in the 48th over and no more runs were added. \\

\begin{figure}
	\centering
	\begin{subfigure}[b]{0.225\textwidth}
		\includegraphics[width=\textwidth]{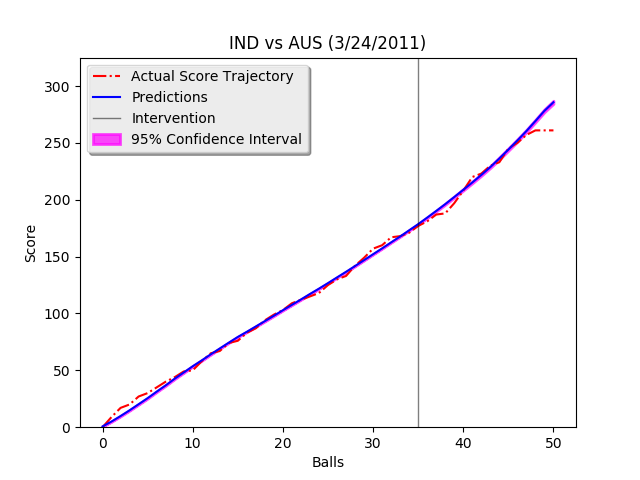}
		\label{fig:ind-aus-2-25}
	\end{subfigure}
	\begin{subfigure}[b]{0.225\textwidth}
		\includegraphics[width=\textwidth]{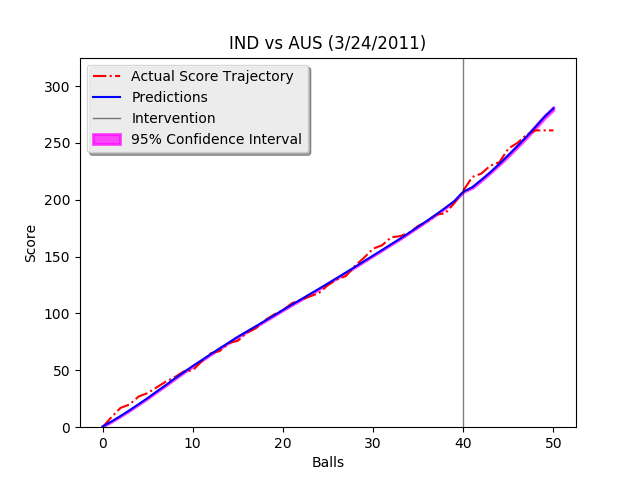}
		\label{fig:ind-aus-2-40}
	\end{subfigure}
	\begin{subfigure}[b]{0.225\textwidth}
		\includegraphics[width=\textwidth]{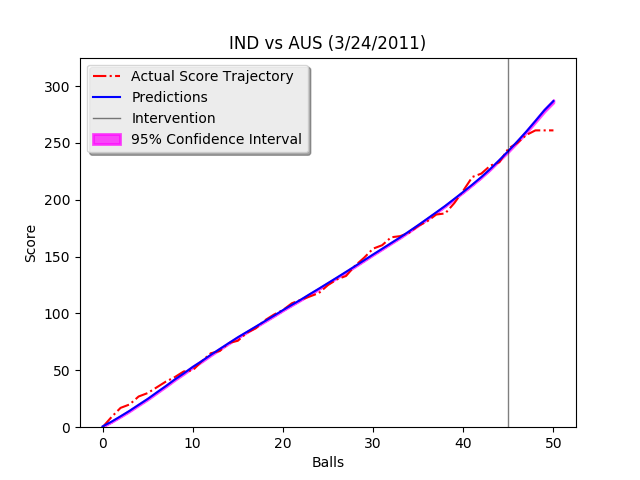}
		\label{fig:ind-aus-2-45}
	\end{subfigure}
	\caption{India vs Aus (WC 2011). Second Innings (India batting). Interventions at the 35, 40 and 45 over marks. Actual and Forecast trajectories with the 95\% uncertainty interval.}
	\label{fig:aus-ind-2}
\end{figure}

\textbf{Zimbabwe vs Australia, Feb 4 2001.} Zimbabwe and Australia played a LOI game in Perth in 2001. Australia, world champions then, were considered too strong for Zimbabwe and batting first made a well-above par 302 runs for the loss of only four wickets. The target was considered out of Zimbabwe's reach. Zimbabwe started poorly and had made only 91 for the loss of their top three batsmen by the 19th over. However, Stuart Carlisle and Grant Flower combined for a remarkable partnership to take Zimbabwe very close to the finish line. Eventually, Australia got both batsmen out just in the nick of time and ended up winning the game by just one run. We show the forecast trajectories at the 30, 35, 40 and 45 over marks--all during the Carlisli-Flower partnership. The forecasts track reality quite well. A key feature to highlight here is the smoothness of the forecasts (in blue) compared to reality (in red). This is a key feature of our algorithm which ``de-noises'' the data matrix to retain only the top few singular values. The resulting smoothness is the mean effect we are trying to estimate and it is no surprise that the forecast trajectories bring this feature to light.

\begin{figure}
	\centering
	\begin{subfigure}[b]{0.225\textwidth}
		\includegraphics[width=\textwidth]{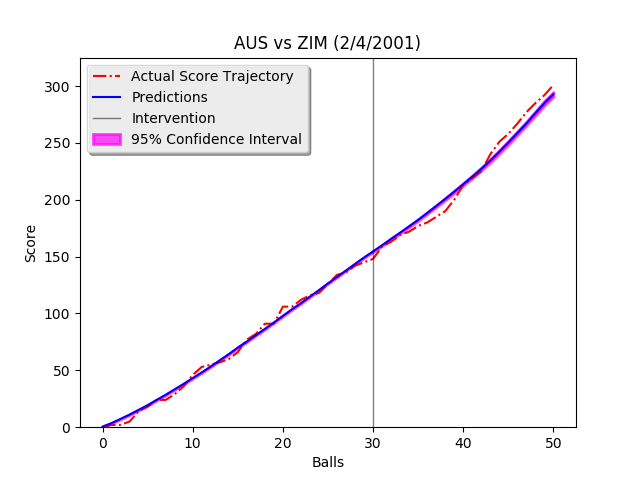}
		\label{fig:zim-aus-2-30}
	\end{subfigure}
	\begin{subfigure}[b]{0.225\textwidth}
		\includegraphics[width=\textwidth]{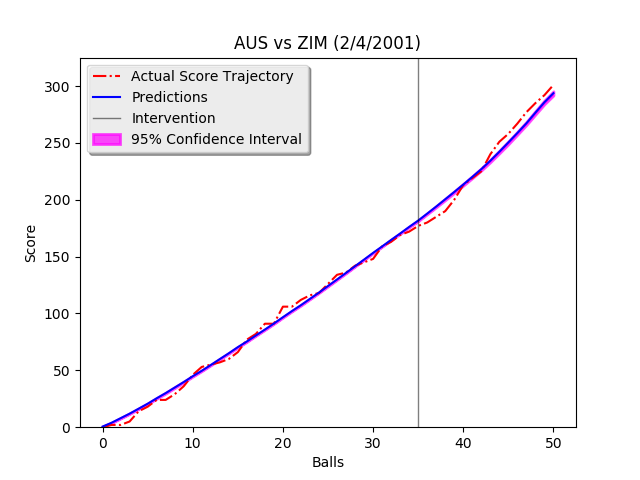}
		\label{fig:zim-aus-2-35}
	\end{subfigure}
	\begin{subfigure}[b]{0.225\textwidth}
		\includegraphics[width=\textwidth]{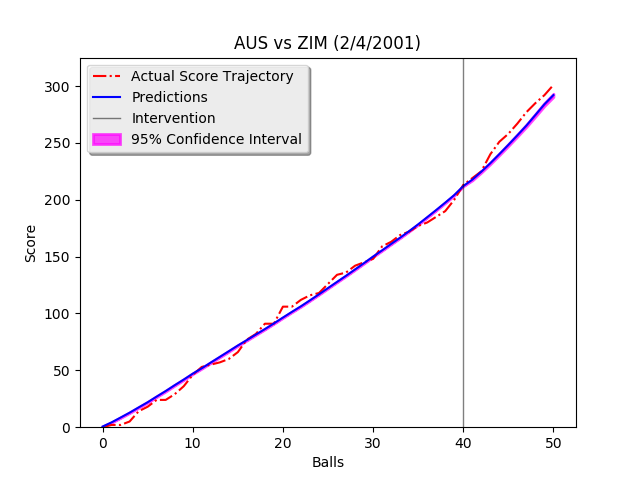}
		\label{fig:zim-aus-2-40}
	\end{subfigure}
	\begin{subfigure}[b]{0.225\textwidth}
		\includegraphics[width=\textwidth]{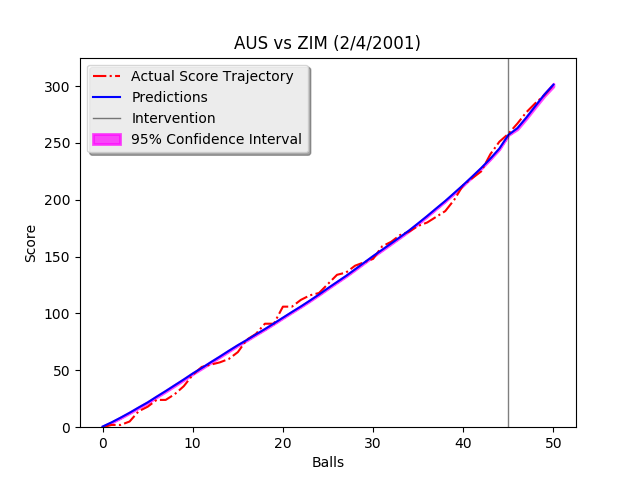}
		\label{fig:zim-aus-2-45}
	\end{subfigure}
	\caption{Zimbabwe vs Aus (2001). Second Innings (Zimbabwe batting). Interventions at the 30 over, 35 over, 40 over and 45 over mark.}
	\label{fig:aus-zim-2}
\end{figure}

\section{Target Resetting Algorithm: Case Studies Continued} \label{sec:appendix_target_resetting_casestudies}
We consider the famous World Cup 2003 game between South Africa and Sri Lanka. South Africa were chasing a target of 269 in 50 overs (300 balls). Rain made an appearance during the second innings and it became clear that at the end of the 45th over (270th ball) of the chase, no more play would be possible. Mark Boucher, a senior player in the South African team, was provided the Duckworth-Lewis-Stern (DLS) par score for the end of the 45th over and hit six runs off the penultimate ball before the intervention (anticipating play to halt at the end of the over since it had started raining). With that six, South Africa had achieved the par score and Boucher blocked the next ball for zero runs (and importantly, did not lose his wicket). South Africa walked off confident that they had achieved the DLS-revised target to win the game. However, they were informed that the ``par'' score they were provided was the DLS-revised score to \textit{tie} the game and they needed one more than par to win!  Unfortunately for South Africa, that tie meant they were knocked out of the world cup which they were also hosting in the most cruel of manners, as noted by The Guardian (\cite{dls-par-1}). 

%We use this game to illustrate how our method would work under Scenario 1. Firstly, we introduce a hypothetical intervention at the 30th over (180 balls) mark and compute the revised target and the corresponding scaled 10-wicket score by South Africa beyond the intervention.  Figure \ref{fig:saf-sri-30} illustrates that scenario. Up until that point, the team was expected to be chasing the original target of in 50 overs (300 balls). The green trajectory is the average path to victory while the red trajectory is the $w_{max} = 10$ wickets target for each point in the innings for $j > b_1 = 180$. The actual innings is shown by the black line. The trajectory in pink is the $\boldsymbol{g}(., .)$ transformed actual trajectory of the runs scored for $j > b_1 = 180$. For each ball, $b_1 < j \leq 300$, South Africa would be declared the winner whenever the pink line was above the red line, and no more play was possible. We note that after the 30 over mark, the red and pink trajectories remain very close to each other which accurately reflects the state of the chase where it was neck-and-neck after the 30th over with South Africa having lost three wickets in the space of seven overs after looking set for victory up until the 23rd over.

We also use Figure \ref{fig:saf-sri-revised} to illustrate how our method would have decided the result of the game at the \textit{actual} intervention which happened at the 45 over mark when no more play was possible. At precisely the 270 ball mark, the revised target score (for having lost 6 wickets) produced by our algorithm was 232. The score made by South Africa was 229 (for the loss of 6 wickets). Therefore, our algorithm would have declared Sri Lanka to be the winner--by a margin of two runs. This is an example that hints that the DLS method might be setting the revised target a touch too low (leading to a bias in favor of the chasing teams).

\begin{figure}
	\centering
	\includegraphics[width=0.3\textwidth]{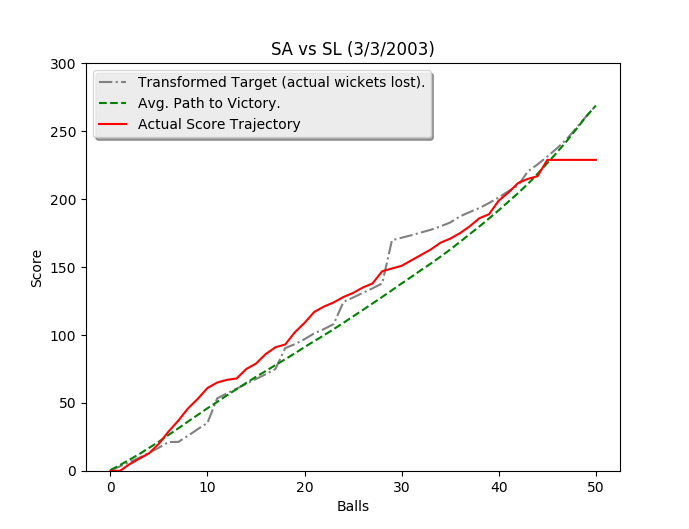}
	\caption{Actual Intervention at 45 overs (270 balls) and no more play was possible after. New Zealand's actual innings (solid red), average path to victory (dashed green) and revised target (dotted-dashed gray)}
	\label{fig:saf-sri-revised}
\end{figure}
